# Supplementary material for: Fuzzy Fault Trees Formalized
Source: arXiv:2403.08843 source file (2024-03-13)
Supplement: Supplementary file 1 [file appendix.tex]

\section*{Appendix}

\begin{table}\label{tab:mix_possibilities}
\caption{Type of each BE when combining triangular, trapezoidal, Gaussian possibilities to BEs.}\label{tab1}
\begin{tabular}{l|l|l}
% \hline
 % &  CSD & LSTF\\
\backslashbox{Type}{Model}  &  CSD & LSTF\\
\hline
tri & B006, B003 & B1-1, B2-1-1, B2-2-1, B2-3, B3-1, B4-1-1, B5-1-1, B5-2-2 \\ 
trap & B005, B006 & B1-2, B2-1-2, B3-2, B4-1-2, B4-2-1, B5-1-2, B5-3-1\\
Gauss & B001, B007 & B1-3, B2-2-2, B3-3, B4-1-3, B4-2-2, B5-2-1, B5-3-2
\end{tabular}
\end{table}
